# Supplementary material for: A Compilation Target for Probabilistic Programming Languages
Source: arXiv:1403.0504 source file (2014-07-10)
Supplement: Supplementary file 1 [file appendix.tex]

% !TEX root = ../main.tex

\begin{figure*}[p!]
\centering
\begin{lstlisting}
// Polya urn (Chinese restaurant process)
typedef struct {
    double concentration;
    int len_buckets;
    int max_buckets;
    int sum_counts;
    int *counts;
} polya_urn_state;

/**
 * Create a polya urn with specified concentration
 *
 */
void polya_urn_new(polya_urn_state *state, double concentration) {
    int s = 2; // initial size
    *state = (polya_urn_state) { concentration, 0, s, 0, malloc(s*sizeof(int)) };
}

/**
 * Clear polya urn state, free internal memory usage
 *
 */
void polya_urn_free(polya_urn_state *state) {
    free(state->counts);
}

/**
 * Draw a number from an existing urn
 *
 */
int polya_urn_draw(polya_urn_state *state) {
    // expand internal state if necessary
    if (state->len_buckets == state->max_buckets) {
        state->max_buckets *= 2; // growth factor
        state->counts = realloc(state->counts, state->max_buckets*sizeof(int));
    }
    
    // draw from urn
    if (state->len_buckets == 0) {
        // first draw
        state->counts[0] = 1;
        state->len_buckets = 1;
        state->sum_counts++;
        return 0;
    } else {
        // subsequent draws
        double *sampling_dist = malloc((1+state->len_buckets)*sizeof(double));
        for (int i=0; i<state->len_buckets; i++) {
            sampling_dist[i] = (double)state->counts[i] / (state->concentration + state->sum_counts);
        }
        sampling_dist[state->len_buckets] = state->concentration / (state->concentration + state->sum_counts);
        
        // draw
        int bucket = discrete_rng(sampling_dist, state->len_buckets+1);
        free(sampling_dist);

        // update counts
        if (bucket < state->len_buckets) {
            state->counts[bucket]++;
        } else {
            state->counts[bucket] = 1;
            state->len_buckets++;
        }
        state->sum_counts++;
        return bucket;
    }
}
\end{lstlisting}
\caption{Polya urn scheme. (Appendix)}
\end{figure*}
